# Supplementary material for: EvoMisty: Building, Optimizing, and Evolving Capabilities on a Social Robot
Source: arXiv:2611.31341 source file (2026-11-27)
Supplement: Supplementary file 1 [file X_suppl.tex]

\clearpage
\setcounter{page}{1}
\maketitlesupplementary

\setcounter{section}{0}
\renewcommand{\thesection}{\Alph{section}}
\makeatletter
\@ifundefined{theHsection}{}{\renewcommand{\theHsection}{supp.\Alph{section}}}
\makeatother

\renewcommand{\dblfloatpagefraction}{0.7}
\makeatletter
\setlength{\@dblfptop}{0pt}
\setlength{\@dblfpsep}{\dblfloatsep}
\setlength{\@dblfpbot}{0pt plus 1fil}
\makeatother

This supplementary material contains details on capability verification in Build (\cref{sec:supp-build}), the measurements and program changes in Optimize together with optimization without EvoMisty (\cref{sec:supp-optimize}), skill distillation and reuse in Evolve (\cref{sec:supp-evolve}), the 28 tasks of the AutoMisty benchmark (\cref{sec:supp-benchmark}),the seven new tasks (\cref{sec:supp-newtasks}), the three accompanying videos (\cref{sec:supp-videos}) and ethical considerations(\cref{sec:supp-ethics}).
\input{sec/supp_A_build}
\input{sec/supp_B_optimize}
\input{sec/supp_C_evolve}
\input{sec/supp_D_benchmark}
\input{sec/supp_E_newtasks}
\section{Supplementary Videos}
\label{sec:supp-videos}
Three videos recorded on the physical robot accompany this document. \suppcode{Naughty\_Child\_Dialogue.mp4} and \suppcode{External\_Camera\_Line\_Following.mp4} compare the programs for Task~\supptaskref{supp:task25}{25} and Task~\supptaskref{supp:taskN6}{N6} before and after optimization, side by side. \suppcode{Minimal\_Pair\_Therapy.mp4} shows a complete robot-led teaching session (Task~\supptaskref{supp:taskN7}{N7}).
\input{sec/supp_F_ethics}
