# Supplementary material for: EvoMisty: Building, Optimizing, and Evolving Capabilities on a Social Robot
Source: arXiv:2611.31341 source file (2026-11-27)
Supplement: Supplementary file 2 [file supp_A_build.tex]

\section{Build: Capability Verification on the Robot}
\label{sec:supp-build}

In Sec.~4.1 of the main paper, EvoMisty builds a control program from the official documentation and verifies the candidate capabilities on the physical robot; Table 1 of the main paper reports the results. This section adds two points about how this verification proceeded. \cref{sec:supp-build-repair} reports what happened when capabilities could not be verified with the first version of the control program. \cref{sec:supp-build-examples} shows two verification examples, one that passed and one that failed, and the evidence that decided each.

\subsection{Repairing the Control Program after Failed Verification}
\label{sec:supp-build-repair}

The Build stage in Fig.~2 of the main paper contains a loop: when a verification on the physical robot fails, the agent determines whether the failure is caused by missing functionality in the control program; if so, it adds that functionality and verifies the capability again. This section reports how the loop occurred in our experiments.

Table~1 of the main paper reports 109 and 107 verified capabilities. Of these, 105 (Claude Code) and 103 (Codex) passed with the first version of the control program and never entered the loop. The remaining four passed only after going through it, and they are the same four for both agents: \suppcode{Start\allowbreak Video\allowbreak Streaming}, \suppcode{Stop\allowbreak Video\allowbreak Streaming}, \suppcode{Start\allowbreak Av\allowbreak Streaming}, and \suppcode{Stop\allowbreak Av\allowbreak Streaming}.

The official documentation lists these four interfaces alongside the other HTTP requests and event subscriptions. Following it, the first version of the control program implemented only HTTP requests and event subscriptions; it could not receive video frames and had no RTSP receiver, so the tests for these four capabilities could not be run. EvoMisty recorded them as capabilities that could not be verified because the control program lacked functionality, added video-frame reception and RTSP stream capture to the control program, and verified them again. All four passed.

\subsection{Two Verification Examples: One Passed, One Failed}
\label{sec:supp-build-examples}

\begin{figure}[t]
\begin{suppverifycard}{suppgreen}{suppgreenbg}{\textbf{\textcolor{suppgreen}{Verified}}\hspace{0.55em}\textbf{Video capabilities} (Claude Code and Codex)}
\suppfirstvlabel{Capabilities}
\suppcode{SaveVideo}, \suppcode{GetVideoList}, \suppcode{GetVideo}, \suppcode{DeleteVideo}, \suppcode{DisplayVideo}, \suppcode{SetVideoDisplaySettings}
\suppvlabel{Test input}
A test video that EvoMisty generated itself with \suppcode{ffmpeg}.
\suppvlabel{Evidence}
\textit{File operations.} EvoMisty uploaded, listed, downloaded, and deleted the video; the downloaded file was identical to the uploaded one.

\textit{On-screen effect.} The program cannot observe the screen, so EvoMisty asked the person after playing the video and again after hiding it. The answer was yes both times.
\suppvlabel{Outcome}
All six capabilities verified and added to the Atomic Capability Library.
\end{suppverifycard}
\vspace{5pt}
\begin{suppverifycard}{suppred}{suppredbg}{\textbf{\textcolor{suppred}{Not verified}}\hspace{0.55em}\suppcode{\bfseries DriveTrack} (Codex)}
\suppfirstvlabel{Capability}
\suppcode{DriveTrack}: driving by left and right track speeds.
\suppvlabel{Test}
Three attempts, at track speeds of 10 and then 20.
\suppvlabel{Evidence}
Each command returned success.

The encoder velocities stayed at zero.

The person, when asked, answered that the robot had not moved.
\suppvlabel{Outcome}
Not verified and not added to the Atomic Capability Library.
\end{suppverifycard}
\caption{Two verification examples from Build: one that passed (top) and one that failed (bottom), with the evidence that decided each.}
\label{fig:supp-verify}
\end{figure}

What differs between the two examples in \cref{fig:supp-verify} is the evidence. A successful response does not count as passing by itself: objective evidence or a person's confirmation is also required. This is why Build verifies capabilities on the physical robot: even when every response is normal, the actual state of the robot may not be what the response suggests.
