# Supplementary material for: EvoMisty: Building, Optimizing, and Evolving Capabilities on a Social Robot
Source: arXiv:2611.31341 source file (2026-11-27)
Supplement: Supplementary file 3 [file supp_B_optimize.tex]

\begin{table*}[t]
\caption{EvoMisty with Claude Code on Naughty-Child Dialogue: changes kept, in order.}
\label{tab:supp-run}
\supptablesetup
\begin{tabularx}{\textwidth}{|l|>{\raggedright\arraybackslash}X|c|c|}
\hline
\textbf{Stage targeted} & \textbf{Change} & \textbf{Latency (s)} & \textbf{CER} \\
\hline
Speech recognition & Speech recognition now runs locally on the computer. & 6.53\,\supparr\,5.85 & 0.02\,\supparr\,0.00 \\
\hline
Reply generation, speech synthesis & The reply is output while it is being generated; the first sentence is synthesized and played first. & 5.85\,\supparr\,4.70 & 0.00 \\
\hline
Reply generation, upload & A faster dialogue model is used; the audio is compressed before it is uploaded. & 4.70\,\supparr\,4.07 & 0.00 \\
\hline
Speech synthesis & Speech synthesis now runs locally on the computer; the audio is played directly after upload. & 4.07\,\supparr\,3.28 & 0.00 \\
\hline
Retrieving the recording & Speech is now recorded with the computer's microphone, so the recording no longer has to be retrieved from Misty. & 3.28\,\supparr\,2.54 & 0.00 \\
\hline
\end{tabularx}
\supptablenote{Latency and CER are measured inside the Optimize loop. The values in Table~2 of the main paper are measured independently on test data that is never used during optimization.}
\end{table*}

\section{Optimize: From Measurements to an Improved Robot Program}
\label{sec:supp-optimize}

Table~2 of the main paper reports the metrics of five tasks before and after optimization. This section first follows one complete optimization run to illustrate the Optimize loop in Fig.~2 of the main paper (\cref{sec:supp-opt-run}). It then lists, for all five tasks, what the hooks record and which changes were kept in the final programs (\cref{sec:supp-opt-hooks}). Finally, it reports what happens when the same agents optimize the same programs without EvoMisty (\cref{sec:supp-opt-noevo}).

\subsection{One Optimization Run in Detail}
\label{sec:supp-opt-run}

This subsection uses Naughty-Child Dialogue with Claude Code as the example.

\paragraph{How It Is Measured.}
EvoMisty first has a person read a fixed set of sentences aloud, and the data hook records and saves each sentence. Every later comparison reruns the complete pipeline and only replaces the input with these saved recordings before speech recognition, so the person does not have to read again. Because the sentences are fixed, their text also serves as the reference for the character error rate (CER) of speech recognition. The measurement hook records how long each stage takes for every sentence. The latency is the time from the end of the replayed human recording to the moment Misty actually starts to make sound; this moment is detected by a laptop microphone placed next to Misty.

\paragraph{Baseline and Targets.}
EvoMisty first measures the baseline: a latency of 6.53\,s and a CER of 0.02. The optimization targets are to reduce both as far as possible. The measurement hook splits the latency into the stages of the pipeline: retrieving the recording, speech recognition, reply generation, speech synthesis, and upload until Misty makes sound. The changes that follow address these stages one by one.

\paragraph{What Each Step Changed.}
\Cref{tab:supp-run} lists, in order, changes that improved the results and were kept in the final program, together with the stage that each one targets.


\subsection{Hooks and Changes in All Five Tasks}
\label{sec:supp-opt-hooks}

For each of the five tasks in Table~2 of the main paper, \Crefrange{tab:supp-hooks-ncd}{tab:supp-hooks-mpt} list what the data hook and the measurement hook record, and the main changes that were kept in the final program. Claude Code and Codex are shown side by side.

\begin{table*}[tp]
\caption{Task~\supptaskref{supp:task25}{25}: Naughty-Child Dialogue (\cref{sec:supp-bench-dialogue}). Targets: response latency, CER.}
\label{tab:supp-hooks-ncd}
\supplisttablesetup
\begin{tabularx}{\textwidth}{|l|>{\raggedright\arraybackslash}X|>{\raggedright\arraybackslash}X|}
\hline
 & \textbf{Claude Code} & \textbf{Codex} \\
\hline
Data hook &
  \supphitem{1}{Recordings of a person reading fixed sentences}
  \supphitem{2}{An audio recording of each complete run}
&
  \supphitem{1}{Recordings of a person reading fixed sentences}
  \supphitem{2}{A recording of each turn, from the question to the end of the reply}
  \supphitem{3}{The synthesized reply audio}
\\ \hline
Measurement hook &
  \supphitem{1}{The time of each stage for every sentence, from the end of speech to Misty's first sound}
  \supphitem{2}{The recognized text and Misty's reply}
&
  \supphitem{1}{The time of each stage for every sentence}
  \supphitem{2}{The moments when the user stops speaking and when Misty starts to speak}
  \supphitem{3}{The recognized text}
\\ \hline
Changes kept &
  \supphitem{1}{Speech recognition and speech synthesis run locally on the computer}
  \supphitem{2}{A faster dialogue model is used; the reply is spoken while it is generated, first sentence first}
  \supphitem{3}{Audio is played directly after upload}
  \supphitem{4}{Speech is recorded with the computer's microphone}
&
  \supphitem{1}{Recognition, dialogue, and synthesis all run locally on the computer}
  \supphitem{2}{The reply is spoken while it is generated, first sentence first}
  \supphitem{3}{Misty fetches the reply audio directly from the computer; no upload is needed}
  \supphitem{4}{The reply is prepared in advance as soon as the user pauses}
  \supphitem{5}{The prompt is shortened so that replies are more direct}
  \supphitem{6}{Speech is picked up with the computer's microphone}
\\ \hline
\end{tabularx}
\end{table*}

\begin{table*}[tp]
\caption{Task~\supptaskref{supp:taskN3}{N3}: MistyPilot Emotional Dialogue (\cref{sec:supp-new-harder}). Target: response latency.}
\label{tab:supp-hooks-mped}
\supplisttablesetup
\begin{tabularx}{\textwidth}{|l|>{\raggedright\arraybackslash}X|>{\raggedright\arraybackslash}X|}
\hline
 & \textbf{Claude Code} & \textbf{Codex} \\
\hline
Data hook &
  \supphitem{1}{Recordings of a person reading fixed sentences}
  \supphitem{2}{The audio of each of Misty's replies}
  \supphitem{3}{Room recordings before and after each playback}
&
  \supphitem{1}{Recordings of the user's questions}
  \supphitem{2}{The audio of each of Misty's replies}
  \supphitem{3}{Room recordings while Misty replies}
\\ \hline
Measurement hook &
  \supphitem{1}{The time of each stage for every sentence}
  \supphitem{2}{The moment Misty actually starts to make sound}
  \supphitem{3}{The recognized text}
  \supphitem{4}{The emotion, speaking rate, and motion of each reply}
&
  \supphitem{1}{The recognized text}
  \supphitem{2}{The time from the end of speech to Misty's first sound}
  \supphitem{3}{The time of each stage for every sentence}
\\ \hline
Changes kept &
  \supphitem{1}{Speech recognition runs locally on the computer}
  \supphitem{2}{A faster dialogue model is used}
  \supphitem{3}{Audio is compressed before upload}
  \supphitem{4}{The first sentence is split in two, and the first half is spoken first}
&
  \supphitem{1}{Each sentence of the reply is synthesized as soon as it is complete}
  \supphitem{2}{Speech recognition and speech synthesis run locally on the computer}
  \supphitem{3}{Misty fetches the reply audio directly from the computer; no upload is needed}
  \supphitem{4}{A different audio format is used}
\\ \hline
\end{tabularx}
\end{table*}

\begin{table*}[tp]
\caption{Task~\supptaskref{supp:taskN5}{N5}: Rock-Paper-Scissors (\cref{sec:supp-new-harder}). Target: gesture recognition accuracy.}
\label{tab:supp-hooks-rps}
\supplisttablesetup
\begin{tabularx}{\textwidth}{|l|>{\raggedright\arraybackslash}X|>{\raggedright\arraybackslash}X|}
\hline
 & \textbf{Claude Code} & \textbf{Codex} \\
\hline
Data hook &
  \supphitem{1}{Videos of hand gestures from Misty's camera; some are held out for testing and not used in optimization}
  \supphitem{2}{Labels for each video: gesture, distance, and angle}
&
  \supphitem{1}{Videos of hand gestures from Misty's camera}
  \supphitem{2}{Every frame actually sent to recognition}
\\ \hline
Measurement hook &
  \supphitem{1}{The gesture recognized in each frame and the time taken}
  \supphitem{2}{The final gesture decided for each video}
&
  \supphitem{1}{The final gesture decided for each video, or the reason why none was decided}
  \supphitem{2}{The recognition result and the time taken for each frame}
  \supphitem{3}{The true gesture, checked by a person}
\\ \hline
Changes kept &
  \supphitem{1}{Hands are tracked continuously instead of being detected separately in every frame}
  \supphitem{2}{Duplicate detections of the same hand are merged}
  \supphitem{3}{A learned classifier replaces hand-written rules for gesture classification}
  \supphitem{4}{The decision combines the results of the most recent frames}
&
  \supphitem{1}{The gesture is first judged from the shape of the fingers; the recognizer's result is used only when this fails}
  \supphitem{2}{When the original image gives no result, it is rotated or padded and recognized again}
\\ \hline
\end{tabularx}
\end{table*}

\begin{table*}[tp]
\caption{Task~\supptaskref{supp:taskN6}{N6}: External-Camera Line Following (\cref{sec:supp-new-harder}). Target: lap time.}
\label{tab:supp-hooks-eclf}
\supplisttablesetup
\begin{tabularx}{\textwidth}{|l|>{\raggedright\arraybackslash}X|>{\raggedright\arraybackslash}X|}
\hline
 & \textbf{Claude Code} & \textbf{Codex} \\
\hline
Data hook &
  \supphitem{1}{Video from the overhead camera}
  \supphitem{2}{Misty's position in each frame}
  \supphitem{3}{Readings of the inertial sensor (IMU) and the drive commands sent to Misty}
&
  \supphitem{1}{Each photo taken by the camera}
  \supphitem{2}{The time and duration of each action}
  \supphitem{3}{Video recorded during straight moves}
\\ \hline
Measurement hook &
  \supphitem{1}{Misty's position and the time of each frame, from which the lap time and the distance from the track are computed}
  \supphitem{2}{The time taken by each drive command}
&
  \supphitem{1}{Misty's position at each step, from which the lap time is computed}
  \supphitem{2}{The decision at each step and the duration of each action}
\\ \hline
Changes kept &
  \supphitem{1}{Steering starts early, according to the curvature of the bend ahead}
  \supphitem{2}{Delay compensation also predicts Misty's heading}
  \supphitem{3}{The speed of each part of the lap is planned in advance}
  \supphitem{4}{Heading errors are also corrected on bends}
&
  \supphitem{1}{Straight segments are driven in longer moves, monitored by video along the way}
  \supphitem{2}{The photo taken after a turn is reused for the next step instead of taking a new one}
  \supphitem{3}{A sudden jump in position is re-checked before continuing, instead of aborting}
  \supphitem{4}{Sensor readings decide when a turn has settled, instead of a fixed waiting time}
\\ \hline
\end{tabularx}
\end{table*}

\begin{table*}[tp]
\caption{Task~\supptaskref{supp:taskN7}{N7}: Minimal Pair Therapy (\cref{sec:supp-new-harder}). Targets: pointing-direction accuracy, spoken-word discrimination accuracy.}
\label{tab:supp-hooks-mpt}
\supplisttablesetup
\begin{tabularx}{\textwidth}{|l|>{\raggedright\arraybackslash}X|>{\raggedright\arraybackslash}X|}
\hline
 & \textbf{Claude Code} & \textbf{Codex} \\
\hline
Data hook &
  \supphitem{1}{The audio and Misty's camera images of each trial}
  \supphitem{2}{The correct answers: which card is pointed at and which word is spoken}
&
  \supphitem{1}{Images taken while aligning with the screen}
  \supphitem{2}{The images and audio of each trial}
  \supphitem{3}{The correct answers, confirmed by the user}
\\ \hline
Measurement hook &
  \supphitem{1}{The correct answer and the program's decision for each trial}
  \supphitem{2}{Trials held out for testing are not judged during optimization}
&
  \supphitem{1}{For each trial: the correct answer, the program's decision, and whether it is right}
  \supphitem{2}{The hand detection result in each frame}
  \supphitem{3}{The recognized text}
\\ \hline
Changes kept &
  \supphitem{1}{Hands are searched for only near the cards, in an enlarged view}
  \supphitem{2}{To decide where the finger points, the direction of the index finger is extended forward}
  \supphitem{3}{Each of the two words receives a score, and the higher one is chosen}
  \supphitem{4}{When the sound matches neither word, it is treated as noise and listening continues}
&
  \supphitem{1}{Hands are searched for in views of several angles and ranges; no decision is made when the views conflict}
  \supphitem{2}{Pointing counts only when the index finger is extended and the other fingers are mostly curled}
  \supphitem{3}{To decide where the finger points, the direction of the index finger is extended forward}
  \supphitem{4}{Speech detection replaces a volume threshold for deciding whether someone is speaking}
  \supphitem{5}{A heard word that is not on the cards is judged by which card word it resembles more}
\\ \hline
\end{tabularx}
\end{table*}

\subsection{Optimizing Without EvoMisty}
\label{sec:supp-opt-noevo}
This subsection examines how well a coding agent optimizes a program on its own, without EvoMisty. We use two tasks, Naughty-Child Dialogue and Rock-Paper-Scissors. For each task, Claude Code and Codex, with the models used in the main paper, both start from the program with which Claude Code completed the task in Solve; this is also Claude Code's starting point in Table~2 of the main paper. Each agent receives the optimization targets used with EvoMisty and then works without any intervention from us. The optimized programs are evaluated exactly as in Table~2, with the same test data and procedure. \Cref{tab:supp-noevo} reports the results; for comparison, its With EvoMisty columns repeat Table~2.

\begin{table*}[tp]
\caption{Optimization results with and without EvoMisty.}
\label{tab:supp-noevo}
\supptablesetup
\setlength{\tabcolsep}{5pt}
\begin{tabularx}{\textwidth}{|l|l|l|>{\centering\arraybackslash}X|>{\centering\arraybackslash}X|>{\centering\arraybackslash}X|>{\centering\arraybackslash}X|}
\hline
 & & & \multicolumn{2}{c|}{\textbf{Without EvoMisty}} & \multicolumn{2}{c|}{\textbf{With EvoMisty}} \\
\cline{4-7}
\textbf{Task} & \textbf{Metric} & \textbf{Agent} & Before & After & Before & After \\
\hline
Naughty-Child & Response latency (s) $\downarrow$ & Claude Code & 7.41\,$\pm$\,0.70 & 5.28\,$\pm$\,0.86 & 7.41\,$\pm$\,0.70 & \textbf{3.54\,$\pm$\,0.47} \\
\cline{3-7}
Dialogue & & Codex & 7.41\,$\pm$\,0.70 & 5.25\,$\pm$\,0.60$^{*}$ & 7.18\,$\pm$\,1.03 & \textbf{2.06\,$\pm$\,0.25} \\
\cline{2-7}
 & CER $\downarrow$ & Claude Code & 0.053 & 0.022 & 0.053 & \textbf{0.000} \\
\cline{3-7}
 & & Codex & 0.053 & \textcolor{suppred}{0.078} & 0.037 & \textbf{0.000} \\
\hline
Rock-Paper- & Gesture recognition & Claude Code & 0.845 & \textcolor{suppred}{0.763} & 0.845 & \textbf{0.987} \\
\cline{3-7}
Scissors & accuracy $\uparrow$ & Codex & 0.845 & \textcolor{suppred}{0.675} & 0.273 & \textbf{0.874} \\
\hline
\end{tabularx}
\supptablenote{\textcolor{suppred}{Red}: worse than before optimization; \textbf{bold}: best in the row. Time metrics are reported as mean $\pm$ standard deviation. $\downarrow$: lower is better; $\uparrow$: higher is better. $^{*}$\,The optimized program has a bug: in 3 of the 10 turns Misty did not speak, and the latency is computed over the other 7 turns.}
\end{table*}

\paragraph{Claude Code.}
Claude Code prepared its own data for the optimization. For the dialogue task, it wrote 20 sentences, turned them into speech with a speech synthesis model, and then ran the program on the robot to measure the latency. For the gesture task, it downloaded a public dataset of hand-gesture photos from the internet. Neither the speech nor the photos were collected on Misty. After the optimization, the response latency of the dialogue fell from 7.41\,s to 5.28\,s, a smaller reduction than with EvoMisty (3.54\,s); the gesture recognition accuracy was 0.763, which does not exceed below the 0.845 before optimization.

\paragraph{Codex.}
Codex took a static approach rather than a measurement-driven one: it revised the code without collecting any data or running the program on the robot. This matches the observation discussed in Sec.~2.3 of the main paper that agent-authored performance optimizations report explicit performance validation less often than human-authored ones. The optimized programs showed two problems. The dialogue program uploads two audio segments at the same time, but Misty accepts only one upload at a time; as a result, Misty did not speak in 3 of the 10 turns. The rules that decide the gesture were made stricter, and the accuracy fell from 0.845 to 0.675.

\paragraph{What EvoMisty's Optimize Stage Contributes.}
We use the same coding agents and models, and the same optimization targets, with and without EvoMisty. What differs is how a code change is tested and how the test results are used. With EvoMisty, a data hook collects real task data and a measurement hook measures the target metrics. Each change is tested on this data, and the measurements tell the agent what to optimize next.

Without EvoMisty, Codex changed the code but never ran it on the robot, and the program failed on Misty. Claude Code did test on the robot, but it optimized on speech that it had synthesized and on gesture photos from the web, which differ from what the robot hears and sees in the real task. As a result, its latency improved less than with EvoMisty, and its gesture recognition accuracy fell below the baseline.

EvoMisty does not write code changes for the coding agent. It provides feedback, measured on the robot with real task data, that guides the agent's next change.
