# Supplementary material for: EvoMisty: Building, Optimizing, and Evolving Capabilities on a Social Robot
Source: arXiv:2611.31341 source file (2026-11-27)
Supplement: Supplementary file 4 [file supp_C_evolve.tex]

\section{Evolve: Skill Distillation and Reuse}
\label{sec:supp-evolve}

In Sec.~4.4.1 of the main paper, EvoMisty distills the optimized program of Naughty-Child Dialogue into skills, and each of the other three dialogue tasks (Math Tutoring, Keyword Story, and Chinese-to-English Translation, \emph{Translation} for short) is solved once without and once with these skills; Table~3 reports the results. The four dialogue tasks follow the same pipeline: speech input, speech recognition, reply generation, speech synthesis, and playback. These steps are called \emph{stages} below. Based on the Skill Library and the final program of each task, this section reports which skills were distilled and how the three tasks use them.

\subsection{Skills Distilled and Reused with Claude Code}
\label{sec:supp-evolve-cc}

\paragraph{Skills Distilled from Naughty-Child Dialogue.}
Distillation produced six skills, which together cover every stage of the dialogue. \Cref{tab:supp-skills-cc} lists them.

\begin{table*}[t]
\caption{Claude Code: distilled skills and their use in the other three dialogue tasks.}
\label{tab:supp-skills-cc}
\supptablesetup
\begin{tabularx}{\textwidth}{|l|>{\raggedright\arraybackslash}X|c|c|c|}
\hline
\textbf{Skill and stage} & \textbf{What it does} & \supptwolinehead{Math}{Tutoring} & \supptwolinehead{Keyword}{Story} & \textbf{Translation} \\
\hline
\suppskillcell{computer\_push\_to\_talk\_mic}{Speech input} & Records push-to-talk audio with the computer microphone; the audio is available as soon as the key is released. & used & used & used \\
\hline
\suppskillcell{sense\_voice\_asr}{Speech recognition} & Recognizes a recording with a local SenseVoice model. & used & used & used \\
\hline
\suppskillcell{streaming\_chat\_reply}{Reply generation} & Keeps the multi-turn history and streams the reply, handing out the first sentence as soon as it is complete. & adapted & -- & -- \\
\hline
\suppskillcell{melo\_tts\_pitched}{Speech synthesis} & Synthesizes pitch-raised Chinese speech with a local MeloTTS model; outputs MP3. & used & used & -- \\
\hline
\suppskillcell{misty\_audio\_player}{Playback} & Uploads audio to Misty, plays it, and waits until playback completes. & used & used & -- \\
\hline
\suppskillcell{misty\_pipelined\_speaker}{Playback} & Synthesizes incoming text segment by segment and plays the segments back to back on Misty; can be interrupted. & used & adapted & -- \\
\hline
\end{tabularx}
\supptablenote{\emph{used}: imported and called, skill code unchanged. \emph{adapted}: not imported; rewritten on the basis of the skill. --: not used.}
\end{table*}

\paragraph{Reuse in the Other Three Dialogue Tasks.}
The three right-hand columns of \Cref{tab:supp-skills-cc} show how the final program of each task uses each skill. The three tasks use the skills selectively, and three cases can be distinguished. First, speech input and speech recognition are the first two stages of the pipeline, and the three tasks have the same needs there. All three tasks use the two corresponding skills, \suppcode{computer\_push\_to\_talk\_mic} and \suppcode{sense\_voice\_asr}, unchanged. Second, the speech synthesis skill \suppcode{melo\_tts\_pitched} synthesizes Chinese speech. Math Tutoring and Keyword Story answer in Chinese and use it together with the two playback skills, \suppcode{misty\_audio\_player} and \suppcode{misty\_pipelined\_speaker}; Translation has to speak English and uses none of the three. Keyword Story has to accompany each segment with expressions and motions when the segment starts to play, so it adapted \suppcode{misty\_pipelined\_speaker}. Third, reply generation is the stage at which the three tasks differ from one another, and no task imports the corresponding skill, \suppcode{streaming\_chat\_reply}, directly. This skill hands out a reply in at most two pieces (the first sentence, then the rest) and always sends the full conversation history. The needs of all three tasks differ from this: Math Tutoring has to explain sentence by sentence, Keyword Story needs an emotion for each segment, and Translation needs no history. Math Tutoring adapted the skill and rewrote the generation part; the other two tasks implemented generation themselves.

\subsection{Skills Distilled and Reused with Codex}
\label{sec:supp-evolve-codex}

\paragraph{Skills Distilled from Naughty-Child Dialogue.}
Distillation produced six skills, covering the stages from speech recognition to playback; audio encoding is a step between speech synthesis and playback. Speech input was not distilled into a skill.

\begin{table*}[t]
\caption{Codex: distilled skills and their use in the other three dialogue tasks.}
\label{tab:supp-skills-codex}
\supptablesetup
\begin{tabularx}{\textwidth}{|l|>{\raggedright\arraybackslash}X|c|c|c|}
\hline
\textbf{Skill and stage} & \textbf{What it does} & \supptwolinehead{Math}{Tutoring} & \supptwolinehead{Keyword}{Story} & \textbf{Translation} \\
\hline
\suppskillcell{sense\_voice\_transcriber}{Speech recognition} & Recognizes a recording with a local SenseVoice model. & used & used & used \\
\hline
\suppskillcell{local\_chat}{Reply generation} & Streams a reply from a local Qwen3-4B model; keeps no history. & used & used & used \\
\hline
\suppskillcell{kokoro\_synthesizer}{Speech synthesis} & Synthesizes Chinese speech with a local Kokoro model and outputs WAV. & used & used & -- \\
\hline
\suppskillcell{speech\_mp3\_encoder}{Audio encoding} & Encodes WAV speech as MP3 and trims the leading silence. & used & used & -- \\
\hline
\suppskillcell{speech\_server}{Playback} & Serves MP3 audio to Misty at a temporary HTTP address on the computer. & indirect & indirect & -- \\
\hline
\suppskillcell{hosted\_audio\_player}{Playback} & Has Misty play the MP3 at that address and waits until playback completes. & used & used & -- \\
\hline
\end{tabularx}
\supptablenote{\emph{used}: imported and called, skill code unchanged. \emph{indirect}: not imported by the task; called by another skill that the task uses. --: not used.}
\end{table*}

\paragraph{Reuse in the Other Three Dialogue Tasks.}
The three right-hand columns of \Cref{tab:supp-skills-codex} show how the final program of each task uses each skill; no task adapted a skill. The three tasks again use the skills selectively, and two cases can be distinguished. First, all three tasks use the speech recognition skill \suppcode{sense\_voice\_transcriber} and the reply generation skill \suppcode{local\_chat} unchanged. The three tasks have the same needs for speech recognition. Their needs for reply generation differ, but \suppcode{local\_chat} only passes the messages to the model and returns its output: it neither splits the reply nor keeps history, and each task handles these itself. Second, the speech synthesis skill \suppcode{kokoro\_synthesizer} synthesizes Chinese speech. Math Tutoring and Keyword Story answer in Chinese and use it together with the encoding and playback skills \suppcode{speech\_mp3\_encoder}, \suppcode{speech\_server}, and \suppcode{hosted\_audio\_player}. Translation has to speak English: it uses none of the four and speaks with Misty's built-in text-to-speech instead. Its version without skills used cloud speech synthesis; this change does not come from a skill.
