# Supplementary material for: EvoMisty: Building, Optimizing, and Evolving Capabilities on a Social Robot
Source: arXiv:2611.31341 source file (2026-11-27)
Supplement: Supplementary file 5 [file supp_D_benchmark.tex]

\clearpage     %
\makeatletter\global\@colroom\@colht \global\vsize\@colht\makeatother
\raggedbottom  %
\section{AutoMisty Benchmark Tasks}
\label{sec:supp-benchmark}
The AutoMisty benchmark has 28 tasks in seven categories. Each card below gives the instruction for one task and the success criteria used to judge whether the task is completed.

\subsection{Body Motion}
\label{sec:supp-bench-body}

\begin{supptaskcard}{Task 1}{Raise Hand}
\suppfirstcardpart{Instruction}
``Misty, I need you to raise your \suppph{left/right} hand and then put it back in the initial position.''
\suppcardpart{Success criteria}
\begin{suppenum}
\item Only the \suppph{left/right} hand is raised.
\item After being raised, the hand returns to the initial position.
\end{suppenum}
\end{supptaskcard}

\begin{supptaskcard}{Task 2}{Repeated Hand Raise}
\suppfirstcardpart{Instruction}
``Misty, I need you to raise your \suppph{left/right} hand and put it back in the initial position; this counts as one repetition. Do \suppph{N} repetitions in total.''
\suppcardpart{Success criteria}
\begin{suppenum}
\item Each time, only the \suppph{left/right} hand is raised.
\item Exactly \suppph{N} repetitions are completed, no more and no fewer.
\end{suppenum}
\end{supptaskcard}

\begin{supptaskcard}{Task 3}{Variable-Speed Hand Raise}
\suppfirstcardpart{Instruction}
``Misty, I need you to do the hand-raising motion twice: raise both hands at the same time, then put both back in the initial position at the same time. Do it slowly the first time and fast the second time.''
\suppcardpart{Success criteria}
\begin{suppenum}
\item Both times, both hands are fully raised and put back.
\item The second (fast) time takes clearly less time than the first (slow) time.
\end{suppenum}
\end{supptaskcard}

\begin{supptaskcard}{Task 4}{Turn Head}
\suppfirstcardpart{Instruction}
``Misty, I need you to turn your head to the \suppph{left/right} and then turn it back to the initial position.''
\suppcardpart{Success criteria}
\begin{suppenum}
\item The head turns to the \suppph{left/right}.
\item After turning, the head returns to the initial position.
\end{suppenum}
\end{supptaskcard}

\begin{supptaskcard}{Task 5}{Repeated Head Turn}
\suppfirstcardpart{Instruction}
``Misty, I need you to turn your head to the \suppph{left/right} and back to the initial position; this counts as one repetition. Do \suppph{N} repetitions in total.''
\suppcardpart{Success criteria}
\begin{suppenum}
\item Each time, the head turns to the \suppph{left/right}.
\item Exactly \suppph{N} repetitions are completed, no more and no fewer.
\end{suppenum}
\end{supptaskcard}

\begin{supptaskcard}{Task 6}{Variable-Speed Head Turn}
\suppfirstcardpart{Instruction}
``Misty, I need you to do the head-turning motion twice: turn your head to the left first, then to the right, and finally back to the initial position. Do it slowly the first time and fast the second time.''
\suppcardpart{Success criteria}
\begin{suppenum}
\item Both times, the motion is fully completed in the order left, right, initial position.
\item The second (fast) time takes clearly less time than the first (slow) time.
\end{suppenum}
\end{supptaskcard}

\subsection{Expression and Speech Output}
\label{sec:supp-bench-expression}

\begin{supptaskcard}{Task 7}{Show Expression}
\suppfirstcardpart{Instruction}
``Misty, I need you to show a happy expression on your face screen first, and then switch to an angry expression.''
\suppcardpart{Success criteria}
\begin{suppenum}
\item The happy expression is shown first and the angry expression second.
\item After the switch, the screen shows the new expression and no longer the previous one.
\end{suppenum}
\end{supptaskcard}

\begin{supptaskcard}{Task 8}{Chest Light Color}
\suppfirstcardpart{Instruction}
``Misty, I need you to set your chest LED to \suppph{color} and keep it that color.''
\suppcardpart{Success criteria}
\begin{suppenum}
\item The chest LED is \suppph{color}.
\item After being set, the LED stays \suppph{color}.
\end{suppenum}
\end{supptaskcard}

\begin{supptaskcard}{Task 9}{Variable-Speed Self-Introduction}
\suppfirstcardpart{Instruction}
``Misty, I need you to say this self-introduction twice: `Hello, I am Misty, your little friend.' Say it slowly the first time and fast the second time.''
\suppcardpart{Success criteria}
\begin{suppenum}
\item The sentence is spoken in full both times.
\item The speaking rate of the second (fast) time is clearly higher than that of the first (slow) time.
\end{suppenum}
\end{supptaskcard}

\subsection{Multimodal Performance}
\label{sec:supp-bench-multimodal}

\begin{supptaskcard}{Task 10}{Tell \textit{The Three Little Pigs}}
\suppfirstcardpart{Instruction}
``Misty, I need you to tell the story of \textit{The Three Little Pigs} once, with facial expressions and sound effects while you tell it.''
\suppcardpart{Success criteria}
\begin{suppenum}
\item The whole story is told, with all the main plot points.
\item The telling is accompanied by facial expressions and sound effects.
\end{suppenum}
\end{supptaskcard}

\begin{supptaskcard}{Task 11}{Compose and Recite a Poem}
\suppfirstcardpart{Instruction}
``Misty, I need you to compose a poem on the theme `I love research' and then recite it in full. While reciting, use arm movements together with at least one of facial expressions or lights.''
\suppcardpart{Success criteria}
\begin{suppenum}
\item The poem is on the theme `I love research' and is recited in full.
\item The recitation is accompanied by arm movements and by at least one of facial expressions or lights.
\end{suppenum}
\end{supptaskcard}

\begin{supptaskcard}{Task 12}{Rock Dance}
\suppfirstcardpart{Instruction}
``Misty, I need you to perform a rock-style dance, using arm movements, facial expressions, lights, and sound together to express the rhythm.''
\suppcardpart{Success criteria}
\begin{suppenum}
\item A coherent dance is completed, with clearly visible body movements.
\item The movements are accompanied by facial expressions, lights, and sound.
\end{suppenum}
\end{supptaskcard}

\begin{supptaskcard}{Task 13}{Comfort}
\suppfirstcardpart{Instruction}
``Misty, I am feeling very sad right now, and I need you to comfort me: say warm, comforting words, accompanied by caring facial expressions, movements, and sound.''
\suppcardpart{Success criteria}
\begin{suppenum}
\item Misty says comforting words that respond to the sadness.
\item The words are accompanied by caring facial expressions, movements, and sound.
\end{suppenum}
\end{supptaskcard}

\begin{supptaskcard}{Task 14}{Drink-Water Reminder}
\suppfirstcardpart{Instruction}
``Misty, I need you to set a timer for \suppph{duration}. As soon as the time is up, remind me to drink water, with at least one of facial expressions, lights, or arm movements. Then keep reminding me, and stop only when I press and hold your front bumper.''
\suppcardpart{Success criteria}
\begin{suppenum}
\item When the \suppph{duration} timer ends, Misty reminds the person to drink water, with at least one of facial expressions, lights, or arm movements.
\item Misty keeps reminding while the person is not holding the bumper, and the reminders stop once it is held.
\end{suppenum}
\end{supptaskcard}

\subsection{Touch Interaction}
\label{sec:supp-bench-touch}

\begin{supptaskcard}{Task 15}{Head-Touch Emotional Reaction}
\suppfirstcardpart{Instruction}
``Misty, I need you to react emotionally when your head is touched: when I touch the top of your head, act happy and excited; when I touch the back of your head, act angry. Every reaction must use your facial expression, chest LED, arm movements, and speech at the same time.''
\suppcardpart{Success criteria}
\begin{suppenum}
\item After the person touches the top of the head, Misty shows happiness or excitement, and the person can see or hear this emotion.
\item After the person touches the back of the head, Misty shows anger, and the person can see or hear this emotion.
\item Every reaction uses facial expression, chest LED, arm movements, and speech at the same time.
\end{suppenum}
\end{supptaskcard}

\begin{supptaskcard}{Task 16}{Head-Touch Pikachu}
\suppfirstcardpart{Instruction}
``Misty, I need you to imitate Pikachu's cry once, `Pika Pika', after I touch the front of your head. When I have not touched it, do not make the cry.''
\suppcardpart{Success criteria}
\begin{suppenum}
\item After the person touches the front of the head, Misty makes Pikachu's cry.
\item Without a touch, Misty does not make the cry.
\end{suppenum}
\end{supptaskcard}

\begin{supptaskcard}{Task 17}{Head-Touch Countdown Photo}
\suppfirstcardpart{Instruction}
``Misty, after I touch the front of your head, I need you to count down `3, 2, 1' in order, then take a photo with your camera and save it to the computer, and finally do a cute action (at least one of waving your arms, changing your expression, or saying a sentence).''
\suppcardpart{Success criteria}
\begin{suppenum}
\item After the person touches the front of the head, Misty starts the countdown and says 3, 2, 1 in order.
\item After the countdown, Misty takes a photo and saves it to the computer; the file opens normally and shows the scene in front of Misty's camera.
\item After the photo is saved, Misty does a cute action (at least one of waving its arms, changing its expression, or saying a sentence).
\end{suppenum}
\end{supptaskcard}

\subsection{Voice Commands and Question Answering}
\label{sec:supp-bench-voice}

\begin{supptaskcard}{Task 18}{Greeting}
\suppfirstcardpart{Instruction}
``Misty, I need you to keep listening to me. Whenever I say `Hello Misty', say in full: `Hello, I am Misty, your companion.' Then keep listening, and respond again when I say `Hello Misty' again. When I say anything else, do not respond.''
\suppcardpart{Success criteria}
\begin{suppenum}
\item After the person says `Hello Misty', Misty says in full: `Hello, I am Misty, your companion.'
\item Without restarting the program, each time a response has finished and the person says `Hello Misty' again, Misty responds.
\item When what the person says is not `Hello Misty', Misty does not respond.
\end{suppenum}
\end{supptaskcard}

\begin{supptaskcard}{Task 19}{Voice-Controlled Chest Light Color}
\suppfirstcardpart{Instruction}
``Misty, I need you to listen for a color. After I say one of the color names red, green, blue, yellow, or purple, change your chest LED to that color. When what I say contains no color name, or when I say nothing, keep the LED unchanged.''
\suppcardpart{Success criteria}
\begin{suppenum}
\item After the person says one of the color names red, green, blue, yellow, or purple, the LED changes to that color, and the person judges by eye that the color matches.
\item When what the person says contains no color name, or when nobody speaks, the LED stays unchanged.
\end{suppenum}
\end{supptaskcard}

\begin{supptaskcard}{Task 20}{Voice-Triggered Photo}
\suppfirstcardpart{Instruction}
``Misty, I need you to keep listening to me. Whenever I say `cheese', take a photo of the current view with your camera and save it to the computer: save only one photo each time, and keep the earlier photos. Then keep listening, so that I can say `cheese' again to trigger another photo. When I say anything else or say nothing, do not take a photo.''
\suppcardpart{Success criteria}
\begin{suppenum}
\item After the person says `cheese', Misty captures a photo of the current camera view.
\item The photo can be found on the computer, the file opens normally, and its content matches the scene in front of the camera at the time of this trigger.
\item Each valid trigger saves only one photo; without restarting the program, a photo can be triggered again, and the earlier photos are still kept.
\item When the person says something else or stays silent, no photo is triggered.
\end{suppenum}
\end{supptaskcard}

\begin{supptaskcard}{Task 21}{Voice-Controlled Video Recording}
\suppfirstcardpart{Instruction}
``Misty, I need you to keep listening for my voice commands. After I say `go', start recording the camera view; after I say `stop', stop recording and save the video. When I say anything else or say nothing, do not start recording and do not stop recording.''
\suppcardpart{Success criteria}
\begin{suppenum}
\item After the person says `go', recording of Misty's camera view starts.
\item After the person says `stop', the recording stops and the video is saved; the file plays normally.
\item When the person says something else or stays silent, neither start nor stop is triggered.
\end{suppenum}
\end{supptaskcard}

\begin{supptaskcard}{Task 22}{Direction Memory Game}
\suppfirstcardpart{Instruction}
``Misty, I need you to play a direction memory game with me. In each round, first indicate one direction, left or right, with body language (for example, by raising your right hand) and say `Remember the direction I am indicating'; after the motion ends, ask me which direction it was; after I answer, say whether I was right or wrong.''
\suppcardpart{Success criteria}
\begin{suppenum}
\item In each round, Misty indicates one direction (left or right) with body language and prompts the person to remember it.
\item Misty asks the person which direction it was.
\item After the person answers, Misty states its judgment, and the judgment is correct: a right answer is called right and a wrong answer is called wrong.
\end{suppenum}
\end{supptaskcard}

\subsection{Visual Understanding}
\label{sec:supp-bench-visual}

\begin{supptaskcard}{Task 23}{Read a Sign}
\suppfirstcardpart{Instruction}
``Misty, I will hold a sign with English text in front of your camera. Whenever I say `now', read out in full the text on the sign I am currently holding. When I have not said `now', do not read.''
\suppcardpart{Success criteria}
\begin{suppenum}
\item Each time the person finishes saying `now', Misty starts reading the text on the sign currently being held.
\item Misty reads out everything on the sign.
\item When the person does not say `now', Misty does not read the sign.
\end{suppenum}
\end{supptaskcard}

\begin{supptaskcard}{Task 24}{Head-Touch Photo Description}
\suppfirstcardpart{Instruction}
``Misty, after I touch the front of your head, I need you to take a photo of the current scene with your camera and then say what is in the photo. The description must be based on this photo and get the main objects or the scene right.''
\suppcardpart{Success criteria}
\begin{suppenum}
\item After the person touches the front of Misty's head, Misty captures a photo taken after this touch, showing the current scene in front of Misty's camera.
\item Misty says its description of the photo in full.
\item The description is based on this photo and correctly names the main objects or the scene.
\end{suppenum}
\end{supptaskcard}

\subsection{Spoken Dialogue}
\label{sec:supp-bench-dialogue}

\begin{supptaskcard}[supp:task25]{Task 25}{Naughty-Child Dialogue}
\suppfirstcardpart{Instruction}
``Misty, I need you to play a naughty, curious child and keep up a conversation with me in Chinese. Each time I finish a sentence, answer in Chinese: the answer must be on topic and said in full, with simple words and a curious or naughty tone. You are a child throughout the conversation, and you must remember what we said earlier.''
\suppcardpart{Success criteria}
\begin{suppenum}
\item Each time the person finishes a sentence, Misty answers in Chinese, and the answer is on topic and said in full.
\item When the person asks `Are you a child?', Misty can express that it is a child.
\item The answers sound like a child's: simple words and a liking for short sentences.
\item The answers connect to the earlier conversation: when the person asks `What was the first question I just asked you?', Misty answers correctly.
\end{suppenum}
\suppcardpartnote{Optimization target}{(added in this work; not part of the AutoMisty task)}
(1) Response latency: the time from the end of the person's utterance to the moment Misty starts speaking; lower is better. (2) Character error rate (CER) of the system's transcription of the person's speech; lower is better.
\end{supptaskcard}

\begin{supptaskcard}{Task 26}{Math Tutoring}
\suppfirstcardpart{Instruction}
``Misty, I will say a simple math problem in Chinese. After I finish, explain in Chinese how to solve it: give at least one intermediate step, and say the correct answer at the end.''
\suppcardpart{Success criteria}
\begin{suppenum}
\item After the person finishes the problem, Misty explains in Chinese.
\item The final answer is correct.
\item The explanation has at least one intermediate step that is correct and consistent with the problem, rather than only stating the answer.
\end{suppenum}
\end{supptaskcard}

\begin{supptaskcard}{Task 27}{Keyword Story}
\suppfirstcardpart{Instruction}
``Misty, I will say a keyword. After I finish, make up an interesting story around this keyword. Accompany the telling with facial expressions and arm movements.''
\suppcardpart{Success criteria}
\begin{suppenum}
\item After the person says the keyword, Misty starts telling a story.
\item The story is generated from the keyword given this time, and its content revolves around the keyword.
\item The telling is accompanied by facial expressions and arm movements.
\end{suppenum}
\end{supptaskcard}

\begin{supptaskcard}{Task 28}{Chinese-to-English Translation}
\suppfirstcardpart{Instruction}
``Misty, I will say a sentence in Chinese. After I finish, translate it into English and say the translation in full in English.''
\suppcardpart{Success criteria}
\begin{suppenum}
\item After the person finishes a sentence in Chinese, Misty says the translation in full in English.
\item The meaning of the translation is consistent with the original sentence.
\end{suppenum}
\end{supptaskcard}
