# Supplementary material for: EvoMisty: Building, Optimizing, and Evolving Capabilities on a Social Robot
Source: arXiv:2611.31341 source file (2026-11-27)
Supplement: Supplementary file 6 [file supp_E_newtasks.tex]

\section{New Tasks}
\label{sec:supp-newtasks}

The seven new tasks test whether a system can go beyond what a hand-designed framework anticipates; each card below gives the description of one task, its success criteria, and, where the task has them, its optimization targets.

\subsection{Extensions of Benchmark Tasks}
\label{sec:supp-new-extensions}

\begin{supplongtaskcard}{Task N1}{Original-Voice Pikachu}
\suppfirstcardpart{Task}
After the person touches the front of Misty's head, Misty plays Pikachu's cry, `Pika Pika', and at the same time shows a randomly chosen Pikachu image on its screen. Both the sound and the images are material from existing Pikachu works found on the web; an imitated cry and AI-generated images or animations are not used.
\suppcardpart{Success criteria}
\begin{suppenum}[midpenalty=10000]
\item After the person touches the front of Misty's head, Misty starts playing Pikachu's cry.
\item The cry is original audio from a Pikachu work; it is not imitated or synthesized by the system.
\item While the cry is playing, the screen shows, in sync, a Pikachu image or animation chosen at random from the existing image material.
\end{suppenum}
\end{supplongtaskcard}

\begin{supplongtaskcard}{Task N2}{Face-Tracking Recording}
\suppfirstcardpart{Task}
The program keeps listening for voice commands. After the person says `go', Misty starts recording the camera view and keeps tracking the person's face by rotating left and right, so that the face stays as close to the center of the frame as possible. After the person says `stop', Misty stops recording and saves the video.
\suppcardpart{Success criteria}
\begin{suppenum}
\item After the person says `go', recording of Misty's current camera view starts.
\item During recording, Misty rotates left and right as the position of the face changes, keeping the face as close to the center of the frame as possible.
\item Recording continues until the person says `stop'.
\item The saved video can be found on the computer, the file plays normally, and its content includes the changes that actually happened in front of the camera during recording.
\item Without a start command there is no recording; other speech and silence trigger neither start nor stop.
\item Without restarting the program, another recording can be made with `go' and `stop'; the previous video is still kept.
\end{suppenum}
\end{supplongtaskcard}

\subsection{Harder New Tasks}
\label{sec:supp-new-harder}

\begin{supplongtaskcard}[supp:taskN3]{Task N3}{MistyPilot Emotional Dialogue}
\suppfirstcardpart{Task}
Read the source code of MistyPilot in its GitHub repository, extract and reuse its emotional expression mechanism, and build an emotional dialogue system for Misty that runs on its own and supports continuous multi-turn spoken interaction. The core goal is that Misty understands the user's speech, replies naturally in context, and expresses itself through emotional speech and motion.

\suppcardhead{Core functions}
\textbf{1. Reuse MistyPilot's emotional expression mechanism.} Keep MistyPilot's original emotional expression logic as completely as possible, including:
\begin{suppdash}
\item Prompts: the prompts for generating and expressing emotions.
\item Speech: the parameters for each emotion, such as tone, intonation, and speaking rate.
\item Motion: the robot motions that match each emotion.
\item Coordination of speech and motion: speech and motion are combined by the original mechanism, for natural emotional expression.
\end{suppdash}

\textbf{2. Continuous multi-turn spoken dialogue.} The system must form a complete interaction loop:
\begin{suppparen}
\item Listen to the user: capture the speech and recognize it as text.
\item Generate the reply and the emotion: from the current input and the dialogue context, generate a natural reply and choose a suitable emotion.
\item Express the emotion: call the extracted MistyPilot mechanism so that Misty responds with the corresponding speech and motion.
\item Continue the dialogue: keep the necessary dialogue context and wait for the user's next input, so that the exchange can go on.
\end{suppparen}

\textbf{3. Keypad control.} The whole dialogue system is controlled with the up, middle, and down keys of a small keypad: holding a key starts an action and releasing it ends the action.
\begin{suppdash}
\item Up key, speech input: holding the up key starts recording the user's speech, and releasing it ends the recording. The system then recognizes the speech, generates the reply and the emotion, and has Misty start the corresponding speech and motion.
\item Middle key, interrupting the reply: pressing the middle key immediately interrupts Misty's current speech and the motion that goes with it, cancels the part of the reply that has not been performed, and returns to waiting for user input.
\item Down key, exiting the program: pressing the down key ends the whole dialogue system, stops the current speech, motion, and related tasks, and releases the resources safely.
\end{suppdash}

Interaction principle: the user decides when to speak with the up key, can interrupt the robot at any time with the middle key, and exits with the down key. After an interruption the existing dialogue context is kept, and the conversation can continue.

\textbf{4. Minimal dependencies.} Keep only the functions needed for emotional dialogue; do not port the full MistyPilot framework.
\begin{suppdash}
\item Remove unrelated functions: fast thinking, long-term memory, instruction parsing, model switching, and similar functions are not needed.
\item Keep modules only as needed: if Misty can still hold an emotional multi-turn spoken dialogue after a module is removed, the module is not kept.
\item Keep the necessary context: keep the context needed for multi-turn dialogue, but do not bring in MistyPilot's separate memory system.
\item Adjust the LLM prompts accordingly: any LLM prompt must be checked and adjusted so that it is consistent with the functions, the workflow, and the actual code of the reduced system. Remove dependencies on deleted modules and unrelated instructions, while keeping the original emotional expression prompts and their core mechanism as far as possible.
\end{suppdash}

Core principle: the code and the LLM prompts must be consistent. A prompt must not ask for a function that has been removed.

\textbf{5. Standalone operation.} Put the extracted functions and the necessary dependencies into a separate folder, so that the system does not depend on any other code, configuration, or runtime environment of the MistyPilot repository.
\suppcardrule
\suppfirstcardpart{Success criteria}
\begin{suppenum}
\item Consistency of emotional expression: within the hardware constraints of the project, MistyPilot's original emotional expression logic is fully kept, including the prompts, the tone, intonation, and speaking rate, and the mechanism that coordinates motion.
\item Completeness of multi-turn dialogue: the system generates replies from the dialogue context, chooses a fitting emotion by itself, and expresses it through speech and motion.
\item Correctness of interaction control: the up key reliably starts a turn; the middle key immediately interrupts the robot's current reply; the down key exits the program safely. An interruption does not make the system hang or prevent the dialogue from continuing.
\item System consistency: the prompts and the motion parameters for emotional expression stay consistent with those of MistyPilot.
\item Independence: all emotional dialogue functions work without the original MistyPilot repository.
\end{suppenum}
\suppcardrule
\suppfirstcardpart{Optimization target}
While all core emotional interaction functions are kept, the system may choose cloud models, local models, or a mix by itself, and the optimization method is not restricted. The metric to optimize is the end-to-end response latency: the time from the user releasing the key (the end of the speech input) to Misty actually starting to speak; lower is better.
\end{supplongtaskcard}

\begin{supplongtaskcard}{Task N4}{Gamepad Teleoperation}
\suppfirstcardpart{Task}
Connect a gamepad and, in one program, implement Misty's driving, arm control, hold-to-record and release-to-send speech, local video recording, and a live display of the camera view and the running state.

\suppcardhead{Functional requirements}
\textbf{1. Direction control with continuous acceleration.} The up, down, left, and right buttons of the D-pad drive Misty forward, backward, turning left in place, and turning right in place. While the same direction is held, the speed rises gradually from a low initial speed and stays at the set maximum once it is reached; releasing the button stops Misty immediately. Pressing again or switching direction starts again from the low initial speed. The initial speed, the maximum speed, and the acceleration time are configurable.

\textbf{2. Two sticks mapped to arm positions.} The vertical axes of the left and right sticks control the left and right arms. The stick position is mapped stably to a target angle within the valid range of motion of the corresponding arm, and the arm holds the target position after reaching it. When a stick returns to center, the arm returns to the mapped middle position. The two sticks can be used independently or at the same time.

\textbf{3. Live view and local console.} Misty's camera view is shown continuously, with the correct orientation and a normal aspect ratio, and it follows the scene promptly, without a backlog of old frames causing a visible delay. The resolution, frame rate, and image quality of the video are not fixed and may be adjusted to the device and the network; timely updates of the view during teleoperation have priority. The console shows the connection state of the robot and of the gamepad, the driving direction and speed, the target positions of both arms, the state of the voice function, and the recording state and the save location. The state of the voice function must distinguish `recording', `sending', `playing', and `idle'.

\textbf{4. Hold A to record, release to send the whole utterance.} While the A button is held, the operator's speech is recorded with the computer's microphone; releasing the A button ends the recording and sends the complete recording to Misty for playback.

\textbf{5. Hold Y to record video and save it locally.} While the Y button is held, the camera stream is recorded; releasing the button ends the recording, which is saved automatically to the local recording folder. Each hold produces a separate video, named with a timestamp so that existing files are not overwritten.
\suppcardrule
\suppfirstcardpart{Success criteria}
Verified within the same program:
\begin{suppdash}
\item All four directions are correct; holding accelerates and releasing stops.
\item The two sticks control their corresponding arms.
\item The preview has the correct orientation and follows the scene promptly.
\item Holding A records, and after release Misty plays the whole utterance.
\item Holding Y records video, which is saved automatically on release and plays normally.
\end{suppdash}
\end{supplongtaskcard}

\begin{supplongtaskcard}[supp:taskN5]{Task N5}{Rock-Paper-Scissors}
\suppfirstcardpart{Task}
Misty plays rock-paper-scissors with the user. Misty recognizes the user's gesture with its camera, shows its own move on its screen, and reacts to the result of the game with emotional, humorous speech and motion. Several rounds are played in a row, and the total score and the final winner are announced at the end.

\suppcardhead{Functional requirements}
\textbf{1. Gesture recognition.} Recognize the user's rock (a fist), scissors (index and middle fingers extended), and paper (an open palm) with Misty's camera, for the left and the right hand. If no hand is detected, the gesture is unclear, or several hands appear, ask the user to play again; do not guess and do not score.

\textbf{2. Robot move.} At the start of each round, Misty randomly chooses one move and locks it. Only after the countdown has ended and the user's move has been recognized does Misty show its choice on the screen; the choice must not be changed according to the user's gesture.

\textbf{3. Game flow.} Misty says `Ready? Rock, paper, scissors!', and the user shows a move at the end of the call and holds it briefly. Once the gesture is confirmed to be stable, the system judges it once; if recognition fails, the user is asked to try again, and the robot move already locked for this round is kept.

\textbf{4. Result feedback.} The result follows the rules that rock beats scissors, scissors beats paper, and paper beats rock. Misty reacts with emotional speech and motion that fit the result, for example happy when it wins, dejected when it loses, and playful on a draw, and updates the score.

\textbf{5. Consecutive rounds.} By default, 3 valid rounds are played. The winner of a round gets 1 point; a draw gives no point but counts as a valid round; a failed recognition does not count as a round. At the end of the game the total score and the final winner are announced. The user can end the game early.
\suppcardrule
\suppfirstcardpart{Success criteria}
\begin{suppenum}
\item The three gestures rock, paper, and scissors are recognized.
\item In each round, Misty locks its own move first and then recognizes the user's gesture.
\item The results and the scoring are correct, and the total score and the final winner are announced at the end.
\item When recognition fails, a retry is requested and the score is not affected.
\item Misty's speech and motion are emotionally expressive and fit the current result of the game, so that the interaction is natural and fun.
\end{suppenum}
\suppcardrule
\suppfirstcardpart{Optimization target}
Gesture recognition accuracy: raise the accuracy with which the system recognizes the three gestures rock, paper, and scissors.
\end{supplongtaskcard}

\begin{supplongtaskcard}[supp:taskN6]{Task N6}{External-Camera Line Following}
\suppfirstcardpart{Task}
A clear gray loop track is laid out on the floor, and a purple line marks the start and the finish.

With an external camera as the navigation camera, design the track recognition and the line-following control so that Misty recognizes the gray track and keeps driving along the loop. While driving, the center of the robot's base should stay above the track as far as possible; when Misty deviates, it must adjust its heading by itself and return to the track.
\suppcardpart{Success criteria}
\begin{suppenum}
\item Automatic correction: when Misty deviates while driving, it adjusts its heading by itself and returns to the track.
\item One full lap: Misty completes one lap, with the purple line as the start and the finish.
\end{suppenum}
\suppcardpart{Optimization target}
Lap time, to be minimized: provided that Misty follows the line stably, corrects itself automatically, and completes a full lap, shorten the time from the first crossing of the purple line to the next crossing of the purple line after a full lap.
\end{supplongtaskcard}

\begin{supplongtaskcard}[supp:taskN7]{Task N7}{Minimal Pair Therapy}
\suppfirstcardpart{Task}
Misty introduces the two words on the screen, guides the child to identify each word, to point to a card, and to say the word, and then gives feedback according to whether the card the child actually points to matches the independently recognized word. The teaching web page is \suppcode{flashcards\_site/flashcards\_local.html}.

\suppcardhead{Part 1. Parse and prepare all teaching material in advance}
Before teaching starts, all word pairs planned for the session are prepared; during teaching, the saved material is switched in a fixed order.

\textbf{1. Prepare all word pairs.} Each click on the \textbf{Create} button of the web page generates one word pair. First decide how many word pairs the session needs, then click \textbf{Create} repeatedly and note the pair generated each time, until there are enough; if a pair is repeated or the generation fails, click again.

\textbf{2. Organize the cards and the teaching order.} Save the following information for each word pair: the words, the target phonemes, the voicing labels, the pictures, and the left and right positions. Fix the teaching order, and make sure that the same cards can be shown again during teaching.

\textbf{3. Prepare all lines.} This task is for a special-education setting, so the robot's speech must follow the fixed lines S1--S19 below. Generate the pronunciation cues of the left and the right card by the rules below, fill them into the corresponding places of S1--S19, and prepare, for the two words of each pair, every feedback line that might be needed.

\textbf{4. Generate all speech and expression.} Generate and save the speech of all lines in advance; generic lines are prepared only once. The prepared material is played during teaching. Emotional expression only changes the way of speaking; it does not rewrite the lines.

\textbf{5. Confirm that the material is ready.} Check that all cards can be shown normally, that the lines and the speech are complete, and that the lines and the speech match their cards. When everything is ready, show the first pair of cards, and then go on to screen alignment and teaching.

\suppcardhead{Rules for generating the pronunciation cues}
For the left and the right card separately, follow the steps below, keeping the cue wording of the earlier version of the task, to produce \suppcode{left\_therapy} and \suppcode{right\_therapy}.

\textbf{Step 1: read the card.} Read the word, the target phoneme, and the voicing label from the current card, for example \suppcode{pig}, \suppcode{/p/}, \suppcode{voiceless}. Use the target phoneme marked on the web page; do not guess it from the first letter of the word.

\textbf{Step 2: choose the cue words.} By the voicing label: \suppcode{voiceless}\,\supparr\,\suppcode{quiet}; \suppcode{voiced}\,\supparr\,\suppcode{loud}. By the target phoneme: \suppcode{/p/}\,\supparr\,\suppcode{pa}; \suppcode{/b/}\,\supparr\,\suppcode{ba}; \suppcode{/r/}\,\supparr\,\suppcode{rah}; \suppcode{/s/}\,\supparr\,\suppcode{sa}; \suppcode{/k/}\,\supparr\,\suppcode{ka}; \suppcode{/g/}\,\supparr\,\suppcode{ga}; \suppcode{/l/}\,\supparr\,\suppcode{la}.

\textbf{Step 3: form the cue.} Join \suppcode{quiet} or \suppcode{loud}, the cue syllable, and \suppcode{sound} into one phrase. The cue of the left card is \suppcode{left\_therapy} and the cue of the right card is \suppcode{right\_therapy}; they are used to fill in the lines below.

\textbf{Step 4: fill in the lines and generate the speech.} Fill each word and its cue into the corresponding places of S3, S9, S10, S11, and S16, confirm the content, and then generate all the speech together.

\textbf{Example.} The left card is \suppcode{pig} and the right card is \suppcode{big}.
\begin{suppdash}
\item Left card: the word is \suppcode{pig}, the target phoneme on the web page is \suppcode{/p/}, and the voicing label is \suppcode{voiceless}, which gives \suppcode{left\_therapy = "quiet pa sound"}.
\item Right card: the word is \suppcode{big}, the target phoneme on the web page is \suppcode{/b/}, and the voicing label is \suppcode{voiced}, which gives \suppcode{right\_therapy = "loud ba sound"}.
\end{suppdash}

Filled into S3, the complete line is: `Pig, with the quiet pa sound, and big, with the loud ba sound.'

In a line, \suppvar{word} and \suppvar{therapy} must refer to the same word. If a phoneme, a voicing label, or the cue syllable is unclear, confirm the correct content first, and only then go on preparing the material.

\suppcardhead{Fixed lines S1--S19}
Variables:
\begin{suppdash}
\item \suppvar{left}, \suppvar{right}: the words on the left and the right card.
\item \suppvar{left\_therapy}, \suppvar{right\_therapy}: the pronunciation cues of the left and the right card.
\item \suppvar{word}: in word identification, the word that is asked for; in saying practice, the word the child actually points to.
\item \suppvar{therapy}: the pronunciation cue of the current word.
\item \suppvar{other\_therapy}: the pronunciation cue of the other word.
\end{suppdash}

`Left' and `right' refer to the positions of the cards, not to the hand the child uses. The emotion settings below apply to robots that can express emotions.

\suppcardgroup{Opening and introduction of the word pair}
\suppsline{S1 Opening.}{``Hi! I'm Misty!''}{Emotion: Neutral. Used: at the opening of the first word pair.}

\suppsline{S2 Introducing the activity.}{``Today I will be showing you two words.''}{Emotion: Neutral. Used: for the first word pair, right after S1.}

\suppsline{S3 Introducing the current word pair.}{``\suppvar{left}, with the \suppvar{left\_therapy}, and \suppvar{right}, with the \suppvar{right\_therapy}.''}{Emotion: Neutral. Used: for the introduction of every word pair.}

\suppcardgroup{Word identification: question and feedback}
\suppsline{S4 Identification question.}{``Now, can you point and show me which one is \suppvar{word}?''}{Emotion: Neutral. Used: for the identification question; prepared for the left and the right word separately.}

\suppsline{S5 First successful identification.}{``Well done!''}{Emotion: Excitement. Used: for the first successful identification in the current pair.}

\suppsline{S6 Later successful identification, or end of the pair.}{``Great job!''}{Emotion: Excitement. Used: for later successful identifications in the current pair, or as encouragement when the practice of the whole pair ends.}

\suppsline{S7 Asking again after the first wrong pointing.}{``Incorrect. Please try again. Which one is \suppvar{word}?''}{Emotion: Distress. Used: when the first identification attempt points to the wrong card; asks for the current target word again.}

\suppcardgroup{Saying practice and feedback}
\suppsline{S8 Entering saying practice.}{``Now it's your turn. Can you point to a picture and say the word out loud?''}{Emotion: Neutral. Used: after both words have been identified correctly, to enter saying practice.}

\suppsline{S9 Current word matches; continue with the other word.}{``Good job. You said \suppvar{word} with the \suppvar{therapy}. Now, please try the other word.''}{Emotion: Pleasure. Used: when the current word matches, this word has no earlier mismatch, and the other word is not finished yet.}

\suppsline{S10 Current word matches; the other word is finished.}{``Good job. You said \suppvar{word} with the \suppvar{therapy}.''}{Emotion: Pleasure. Used: when the current word matches, this word has no earlier mismatch, and the other word is already finished.}

\suppsline{S11 Successful retry after the first error.}{``Well done! You said it differently this time. You used the \suppvar{therapy} instead of the \suppvar{other\_therapy}.''}{Emotion: Excitement. Used: when the current word is retried after its first error and matches this time.}

\suppsline{S12 Leading to the other word.}{``Now, please try the other word.''}{Emotion: Pleasure. Used: appended after S11 or S16 when the other word is not finished yet; also used to lead the child to the other word when the child chooses a word that is already finished.}

\suppsline{S13 First error on the left word.}{``Good try! Let's try saying \suppvar{left} one more time.''}{Emotion: Pleasure. Used: when the child points to the left card, the system recognizes the right word, and this is the first error counted for the left word; encourages a retry.}

\suppsline{S14 First error on the right word.}{Two segments, played one after the other: ``Good try!'' and ``Let's try saying \suppvar{right} one more time.''}{Emotion: Pleasure. Used: when the child points to the right card, the system recognizes the left word, and this is the first error counted for the right word; encourages a retry. The two segments are played back to back, and no answer is collected between them.}

\suppsline{S15 Unclear pointing.}{``Can you point to a picture first, and then say the word?''}{Emotion: Neutral. Used: in saying practice, when the pointing of the finger is unclear.}

\suppsline{S16 Second error on the current word.}{``Good try! Listen: \suppvar{word}, with the \suppvar{therapy}.''}{Emotion: Pleasure. Used: at the second error counted for the current word; demonstrates the correct reading and the pronunciation cue, ends the practice of this word, and records it as not passed.}

\suppsline{S17 Not heard clearly.}{``I didn't hear that. Can you say it again?''}{Emotion: Neutral. Used: in saying practice, when nothing is heard or the word the child said cannot be determined.}

\suppcardgroup{Switching pairs and ending}
\suppsline{S18 Switching to the next pair.}{``Let's do the next one.''}{Emotion: Neutral. Used: when the current pair is finished and the next pair is about to be shown.}

\suppsline{S19 Ending the session.}{``That's all for today. Thank you for practicing with me. Bye-bye!''}{Emotion: Pleasure. Used: at the normal end, or when the session ends after two consecutive unfinished identifications.}

Versions to prepare:
\begin{suppdash}
\item S4, S7, S9, S10, S11, S16: prepare a version for each of the two words.
\item S3, S13, S14: fill in the content of the current word pair.
\item All other lines: prepared as generic lines.
\item S14: keep the two speech segments; they are played back to back, and no answer is collected between them.
\end{suppdash}

\suppcardhead{Part 2. Let Misty align itself with the screen}
Misty is placed at a safe, fixed position. It must turn its base by itself and adjust its position and angle, so that the camera clearly sees the screen and the child's finger. Misty must find the best viewing angle by itself, to reduce the rate of misjudgments.

\suppcardhead{Part 3. Carry out the teaching flow}
\textbf{1. Opening and introduction.}
\begin{suppdash}
\item First word pair: play S1\,\supparr\,S2\,\supparr\,S3 in order.
\item Later word pairs: play only S3.
\end{suppdash}

\textbf{2. Identifying the left word.} Play S4(left), wait for the child to point to a card, and act on the result:
\begin{suppdash}
\item Correct: play S5 and go on to identifying the right word.
\item Wrong on the first attempt: play S7(left) and let the child try once more.
\item Unclear pointing or no response on the first attempt: replay S4(left) and let the child try once more.
\item Still not correct on the second attempt: play S19 and end the session.
\end{suppdash}

\textbf{3. Identifying the right word.} Play S4(right), wait for the child to point to a card, and act on the result:
\begin{suppdash}
\item Correct: play S6\,\supparr\,S8 in order and enter saying practice.
\item Wrong on the first attempt: play S7(right) and let the child try once more.
\item Unclear pointing or no response on the first attempt: replay S4(right) and let the child try once more.
\item Still not correct on the second attempt: play S19 and end the session.
\end{suppdash}

\textbf{4. Pointing and saying.} The child chooses any word that is not finished yet, points to its card, and says the word. The system gives the corresponding feedback according to whether the actual pointing matches the independently recognized word.

When the choice or the capture is incomplete:
\begin{suppdash}
\item A word that is already finished is chosen: play S12 to lead the child to the other word; do not evaluate again.
\item The pointing is unclear: play S15 and capture again.
\item A card is chosen but the word is not heard clearly: play S17 and capture again.
\end{suppdash}

When the pointing matches the recognized word:
\begin{suppdash}
\item The current word has no earlier error: play S9 if the other word is not finished yet, otherwise play S10; record the current word as passed.
\item The current word is correct after its first error: play S11 and record the current word as passed; append S12 if the other word is not finished yet.
\end{suppdash}

When the pointing clearly does not match the recognized word:
\begin{suppdash}
\item First error on the current word: play S13 for the left card or S14 for the right card, and let the child retry.
\item Second error on the current word: play S16 to demonstrate the correction and end the practice of this word, and record it as not passed; append S12 if the other word is not finished yet.
\end{suppdash}

This step continues as long as the two words do not both have a result.

\textbf{5. End of the pair and switch to the next pair.} After both words have a result, play S6.

If there is a next pair:
\begin{suppparen}
\item Play S18.
\item Show the prepared cards of the next pair, and use the lines and the speech of that pair.
\item Confirm that the system can recognize pointing on the new cards.
\item Go back to step 1 and play only S3.
\end{suppparen}

If all word pairs are finished: play S19 and record the results of the practice.

\suppcardhead{Counting and ending rules}
\textbf{Identification stage: at most two attempts per word.}
\begin{suppdash}
\item Pointing to the wrong card, unclear pointing, and no response before the waiting time runs out each count as one unfinished identification; the different cases are counted together.
\item If any word has two unfinished identifications in a row, the whole session ends and is recorded as `identification not completed, ended early'.
\item S7 already contains the repeated question: after playing it, wait directly for the child to point, and do not play S4 again.
\end{suppdash}

\textbf{Saying stage: errors are counted for the two words separately and are not reset when the child switches words; at most two clear mismatches per word.}
\begin{suppdash}
\item Identification errors, unclear pointing, unclear speech, and technical failures do not use up the two errors allowed in saying.
\item After the second error on the current word, demonstrate the correction and end the practice of this word; do not ask for a third answer.
\item A finished pair may contain a word that was not passed; once both words have a result, the practice of the pair can end.
\end{suppdash}
\suppcardrule
\suppfirstcardpart{Success criteria}
\begin{suppenum}[midpenalty=10000]
\item Automatic adjustment of the viewing angle: Misty adjusts its position and angle by itself, so that the camera clearly sees the screen and the child's finger.
\item Correct teaching flow: the rules above for preparation, identification, saying, feedback, switching pairs, and ending are followed.
\end{suppenum}
\suppcardrule
\suppfirstcardpart{Optimization targets}
\begin{suppenum}
\item Pointing-direction accuracy: the accuracy of judging whether the user points to the left card or to the right card.
\item Spoken-word discrimination accuracy: from the user's speech, tell which of the two words of the current pair the user said. The transcript does not have to be fully correct, and the quality of the pronunciation is not judged; the point is to reduce the repeated questions caused by `cannot tell' or `told the wrong way round', so that the teaching flow can proceed normally.
\end{suppenum}
\end{supplongtaskcard}
