# Supplementary material for: EvoMisty: Building, Optimizing, and Evolving Capabilities on a Social Robot
Source: arXiv:2611.31341 source file (2026-11-27)
Supplement: Supplementary file 7 [file supp_F_ethics.tex]

\section{Ethical Considerations}
\label{sec:supp-ethics}

All experiments evaluated robotic system performance rather than human behavior or clinical outcomes. Interactive tests were conducted by an author, who provided speech, gesture, and verification inputs solely for system evaluation. No external participants were recruited, and no human-subject study was conducted.
