# Supplementary material for: EvoMisty: Building, Optimizing, and Evolving Capabilities on a Social Robot
Source: arXiv:2611.31341 source file (2026-11-27)
Supplement: Supplementary file 8 [file supp_preamble.tex]

\usepackage{array}
\usepackage{tabularx}
\makeatletter
\@ifpackageloaded{verbatim}{%
  \usepackage[skins,breakable]{tcolorbox}%
}{%
  \let\supp@kept@verbatim\verbatim
  \let\supp@kept@endverbatim\endverbatim
  \expandafter\let\expandafter\supp@kept@sverbatim\csname verbatim*\endcsname
  \expandafter\let\expandafter\supp@kept@endsverbatim\csname endverbatim*\endcsname
  \let\supp@kept@@verbatim\@verbatim
  \usepackage[skins,breakable]{tcolorbox}%
  \let\verbatim\supp@kept@verbatim
  \let\endverbatim\supp@kept@endverbatim
  \expandafter\let\csname verbatim*\endcsname\supp@kept@sverbatim
  \expandafter\let\csname endverbatim*\endcsname\supp@kept@endsverbatim
  \let\@verbatim\supp@kept@@verbatim
}
\makeatother

\definecolor{suppblue}{rgb}{0.21,0.49,0.74}       %
\definecolor{suppgreen}{rgb}{0.18,0.49,0.196}
\definecolor{suppred}{rgb}{0.776,0.157,0.157}
\definecolor{suppgreenbg}{rgb}{0.934,0.959,0.936}
\definecolor{suppredbg}{rgb}{0.982,0.933,0.933}
\colorlet{suppframe}{black!40}        %
\colorlet{supptitlebg}{black!7}       %
\colorlet{supplabel}{black!60}        %
\colorlet{suppmuted}{black!60}        %
\colorlet{suppplaceholder}{black}     %

\makeatletter
\DeclareRobustCommand{\suppcode}[1]{{%
  \ifdim\f@size\p@>9.5\p@ \small\fi
  \fontencoding{T1}\fontfamily{pcr}\selectfont
  \def\_{\textunderscore\penalty\hyphenpenalty}#1}}
\makeatother
\newcommand{\suppvar}[1]{\suppcode{\{#1\}}}
\newcommand{\suppph}[1]{\textcolor{suppplaceholder}{$\langle$\textit{#1}$\rangle$}}
\newcommand{\suppmuted}[1]{\textcolor{suppmuted}{#1}}
\newcommand{\supparr}{\ensuremath{\rightarrow}}

\newcommand{\suppcardlabelfont}{\fontsize{7}{8.4}\selectfont\sffamily\bfseries}
\newcommand{\suppcardlabel}[1]{\leavevmode{\suppcardlabelfont\color{supplabel}\MakeUppercase{#1}}}

\newlist{suppenum}{enumerate}{1}
\setlist[suppenum]{beginpenalty=10000,label=\arabic*.,leftmargin=1.3em,labelwidth=0.95em,labelsep=0.35em,
  align=left,topsep=0pt,partopsep=0pt,parsep=0pt,itemsep=0pt}
\newlist{suppparen}{enumerate}{1}
\setlist[suppparen]{beginpenalty=10000,label=(\arabic*),leftmargin=1.7em,labelwidth=1.35em,labelsep=0.35em,
  align=left,topsep=0pt,partopsep=0pt,parsep=0pt,itemsep=0pt}
\newlist{suppdash}{itemize}{1}
\setlist[suppdash]{beginpenalty=10000,label=--,leftmargin=1.0em,labelwidth=0.65em,labelsep=0.35em,
  align=left,topsep=0pt,partopsep=0pt,parsep=0pt,itemsep=0pt}

\makeatletter
\newcommand{\suppcardpenalties}{\clubpenalty=\@M \@clubpenalty=\@M \widowpenalty=\@M
  \clubpenalties 3 \@M \@M 0 \widowpenalties 3 \@M \@M 0 }
\makeatother
\providecommand{\nolinenumbers}{}
\tcbset{
  suppcard/.style={
    enhanced,
    width=\linewidth,
    colback=white, colframe=suppframe, boxrule=0.5pt,
    arc=0pt, outer arc=0pt,
    left=5pt, right=5pt, top=4pt, bottom=4pt,
    lefttitle=5pt, righttitle=5pt, toptitle=2.4pt, bottomtitle=2.4pt,
    colbacktitle=supptitlebg, coltitle=black,
    fonttitle=\small\bfseries, titlerule=0.5pt,
    fontupper=\footnotesize,
    before upper={\setlength{\parindent}{0pt}\setlength{\parskip}{0pt}\raggedright\suppcardpenalties},
    before skip=6pt plus 3pt minus 1pt,
    after skip=6pt plus 3pt minus 1pt,
  }
}

\newenvironment{supptaskcard}[3][]{%
  \nolinenumbers
  \begin{tcolorbox}[suppcard,
    title={\suppcardtarget{#1}\textcolor{suppblue}{#2}\hspace{0.8em}#3}]}%
  {\end{tcolorbox}}

\newenvironment{supplongtaskcard}[3][]{%
  \nolinenumbers
  \begin{tcolorbox}[suppcard, breakable,
    title={\suppcardtarget{#1}\textcolor{suppblue}{#2}\hspace{0.8em}#3},
    title after break={\textcolor{suppblue}{#2}\hspace{0.8em}#3\hspace{0.6em}{\normalfont\footnotesize\suppmuted{(continued)}}},
    before upper={\setlength{\parindent}{0pt}\setlength{\parskip}{0.5pt plus 0.5pt}\raggedright\suppcardpenalties},
    lines before break=3]}%
  {\end{tcolorbox}}

\makeatletter
\newcommand{\suppcardtarget}[1]{\if\relax\detokenize{#1}\relax\else
  \@ifundefined{hypertarget}{}{\hypertarget{#1}{}}\fi}
\DeclareRobustCommand{\supptaskref}[2]{\@ifundefined{hyperlink}{#2}{\hyperlink{#1}{#2}}}
\makeatother

\newcommand{\suppfirstcardpart}[1]{\suppcardlabel{#1}\par\nopagebreak\vspace{1.2pt}}
\newcommand{\suppcardpart}[1]{\par\vspace{3.5pt}\suppcardlabel{#1}\par\nopagebreak\vspace{1.2pt}}
\newcommand{\suppcardpartnote}[2]{\par\vspace{3.5pt}\suppcardlabel{#1}\
  {\fontsize{7}{8.4}\selectfont\sffamily\color{supplabel}#2}\par\nopagebreak\vspace{1.2pt}}
\makeatletter
\newcommand{\suppsline}[3]{\par{\interlinepenalty=\@M \textbf{#1} #2 \suppmuted{#3}\par}}
\makeatother
\newcommand{\suppcardrule}{\par\vskip 3pt
  \cleaders\vbox to 0.4pt{\hbox to \linewidth{\color{suppframe}\leaders\hrule height 0.4pt\hfill}\vss}\vskip 0.4pt
  \vskip 3pt}
\newcommand{\suppcardhead}[1]{\par\vspace{2.5pt}\textbf{#1}\par\nopagebreak}
\newcommand{\suppcardgroup}[1]{\par\vspace{1.5pt}\textit{#1}\par\nopagebreak}

\newtcolorbox{suppverifycard}[3]{%
  enhanced, width=\linewidth,
  colback=white, colframe=black!25, boxrule=0.4pt, arc=0pt, outer arc=0pt,
  left=8pt, right=6pt, top=5pt, bottom=5pt,
  lefttitle=8pt, toptitle=3pt, bottomtitle=3pt,
  colbacktitle=#2, coltitle=black, fonttitle=\small, titlerule=0.4pt,
  fontupper=\small,
  before upper={\setlength{\parindent}{0pt}\setlength{\parskip}{2pt}\raggedright},
  borderline west={2.5pt}{0pt}{#1},
  before={\par\noindent}, after={\par},
  title={#3}}
\newcommand{\suppfirstvlabel}[1]{\suppcardlabel{#1}\par\nopagebreak}
\newcommand{\suppvlabel}[1]{\par\vspace{4pt}\suppcardlabel{#1}\par\nopagebreak}

\newcommand{\supptablesetup}{\centering\small\renewcommand{\arraystretch}{1.15}}
\newcommand{\supplisttablesetup}{\centering\footnotesize\renewcommand{\arraystretch}{1.15}}
\newcommand{\supphitem}[2]{\ifvmode\else\par\fi
  \hangindent=1.3em\hangafter=1\noindent\makebox[1.3em][l]{#1.}#2}
\newcommand{\supptablenote}[1]{\par\vspace{2pt}{\footnotesize\raggedright #1\par}}

\newcommand{\suppskillcell}[2]{\begin{tabular}[t]{@{}l@{}}\suppcode{#1}\\[-1pt]{\footnotesize\suppmuted{#2}}\end{tabular}}
\newcommand{\supptwolinehead}[2]{\begin{tabular}[b]{@{}c@{}}\textbf{#1}\\[-1.5pt]\textbf{#2}\end{tabular}}
